# Supplementary material for: Evolving generalist controllers to handle a wide range of morphological variations
Source: arXiv:2309.10201 source file (2024-07-19)
Supplement: Supplementary file 1 [file supplementaryInfo.tex]

\section{Fitness trends during the evolutionary processes}
\begin{figure*}[ht!]
    \centering
    \includegraphics[width=0.55\textwidth]{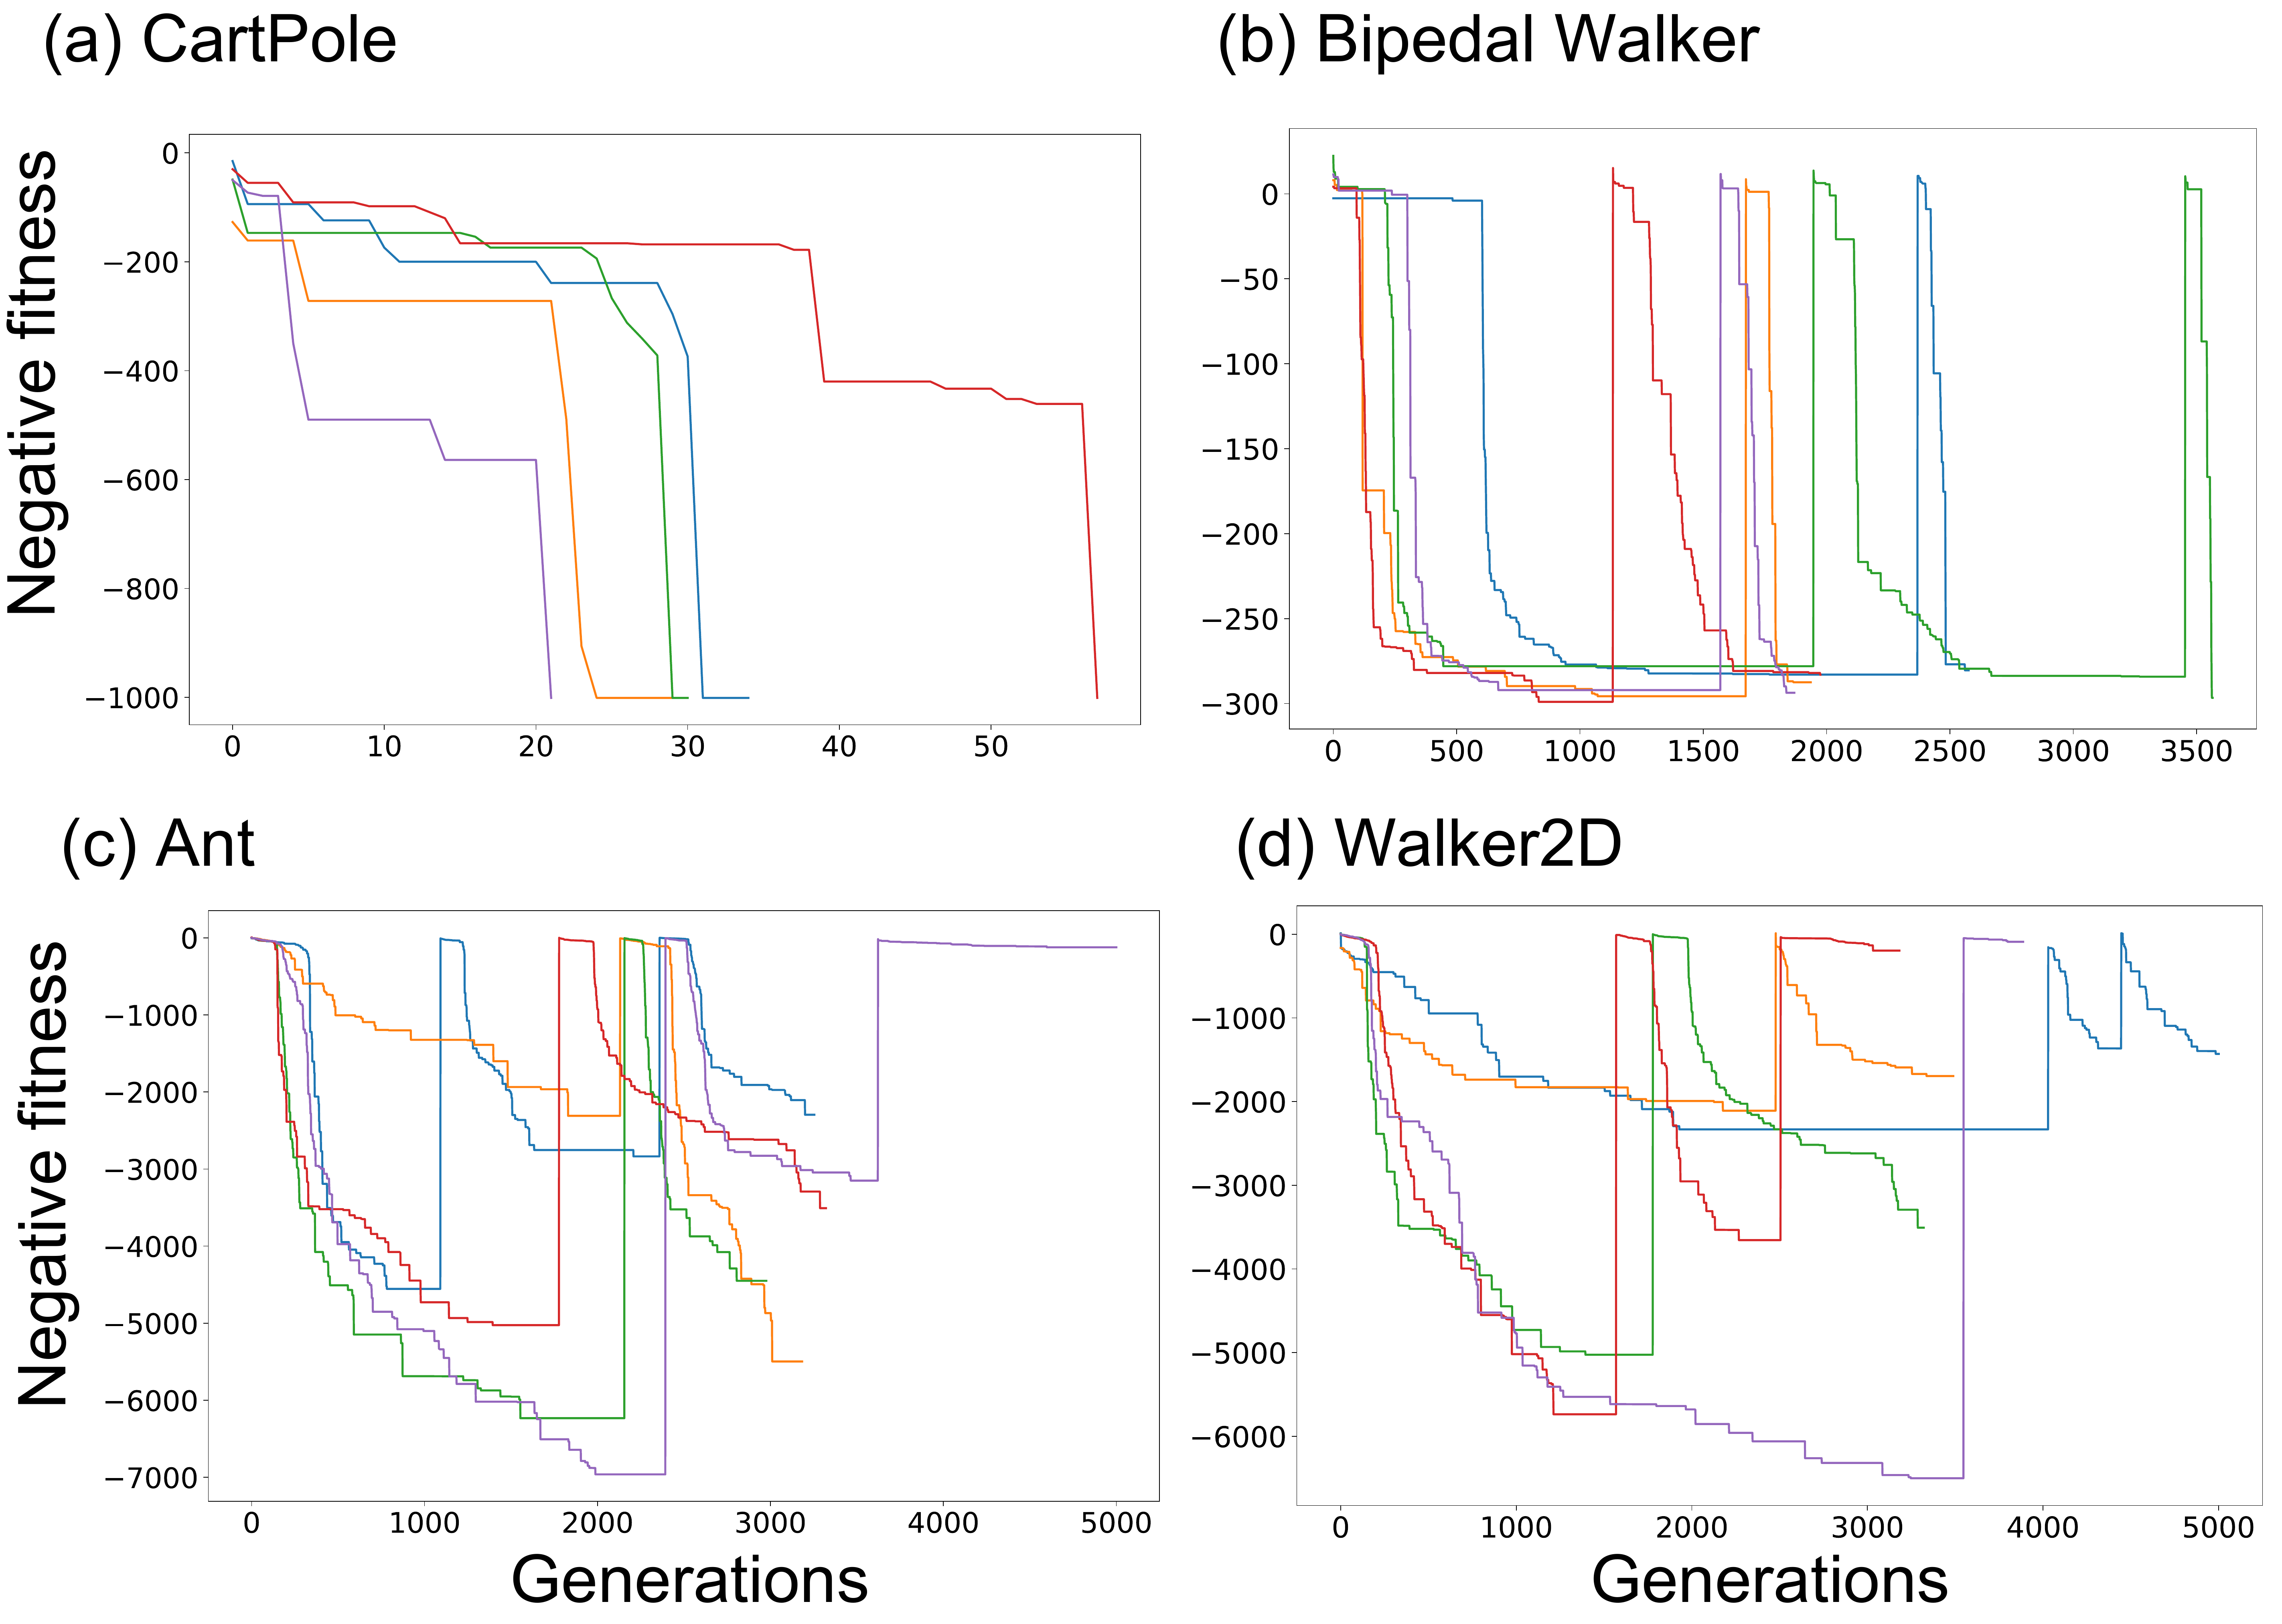}
    \caption{Illustration of fitness values of five independent evolutionary processes (on morphology size of 64) on four problems.}
    \label{fig:evolutionaryRuns}
\end{figure*}

Figure~\ref{fig:evolutionaryRuns} shows the fitness trends during the evolutionary processes on four agent types. In CartPole, evolutionary branching was not observed. A single generalist controller is learned less than 100 generations. In other environments, we can observe occasional fitness increase that indicate the restart of the evolutionary process that is run on the outlier sets. 

\section{Evolutionary branching}
Table~\ref{tab:clusters} shows the average number of evolutionary branching (and standard deviation) observed based on the size of training morphologies in each problem type. CartPole did not show any branching, whereas Walker2D showed the largest number of branching. In Figure~\ref{fig:visual_alg}, illustrate the branching process and how it partitions the space of morphology variations.

\begin{table*}[ht!]
\centering
\caption{Table shows the mean and standard deviation of the number of clusters for each combination of environment and size of the training morphology set.}\label{tab:clusters}
\begin{tabular}{|l|c|c|c|c|c|}
\hline
\begin{tabular}[c]{@{}l@{}}\textbf{Size of training morphologies:}\end{tabular} & \textbf{1} & \textbf{16}  & \textbf{25}  & \textbf{49} & \textbf{64}                                                      \\ \hline
\textbf{CartPole}                                                                                      & \begin{tabular}[c]{@{}c@{}}1 \end{tabular} & \begin{tabular}[c]{@{}c@{}}1   \end{tabular}       & \begin{tabular}[c]{@{}c@{}}1   \end{tabular}        & \begin{tabular}[c]{@{}c@{}}1   \end{tabular}        & \begin{tabular}[c]{@{}c@{}}1   \end{tabular}       \\ \hline
\textbf{Bipedal Walker}                                                                                & \begin{tabular}[c]{@{}c@{}}1   \end{tabular} & \begin{tabular}[c]{@{}c@{}}1.67   $\pm$ 0.96\end{tabular} & \begin{tabular}[c]{@{}c@{}}1.367   $\pm$ 0.56\end{tabular} & \begin{tabular}[c]{@{}c@{}}2.367   $\pm$ 0.61\end{tabular} & \begin{tabular}[c]{@{}c@{}}2.53   $\pm$ 0.78\end{tabular}  \\ \hline
\textbf{Ant}                                                                                          & \begin{tabular}[c]{@{}c@{}}1   \end{tabular} & \begin{tabular}[c]{@{}c@{}}1.67   $\pm$ 0.84\end{tabular} & \begin{tabular}[c]{@{}c@{}}1.7   $\pm$ 0.92\end{tabular}   & \begin{tabular}[c]{@{}c@{}}1.9  $\pm$ 1.12\end{tabular}    & \begin{tabular}[c]{@{}c@{}}2.33   $\pm$ 1.24\end{tabular} \\ \hline
\textbf{Walker2D}                                                                                      & \begin{tabular}[c]{@{}c@{}}1   \end{tabular} & \begin{tabular}[c]{@{}c@{}}2.4   $\pm$ 1.04\end{tabular}   & \begin{tabular}[c]{@{}c@{}}2.9   $\pm$ 0.99\end{tabular}   & \begin{tabular}[c]{@{}c@{}}3.2   $\pm$ 1.06\end{tabular}   & \begin{tabular}[c]{@{}c@{}}3.1   $\pm$ 1.24\end{tabular}  \\ \hline
\end{tabular}
\end{table*}

\begin{figure*}[!ht]
    \centering
    \includegraphics[width=.8\linewidth]{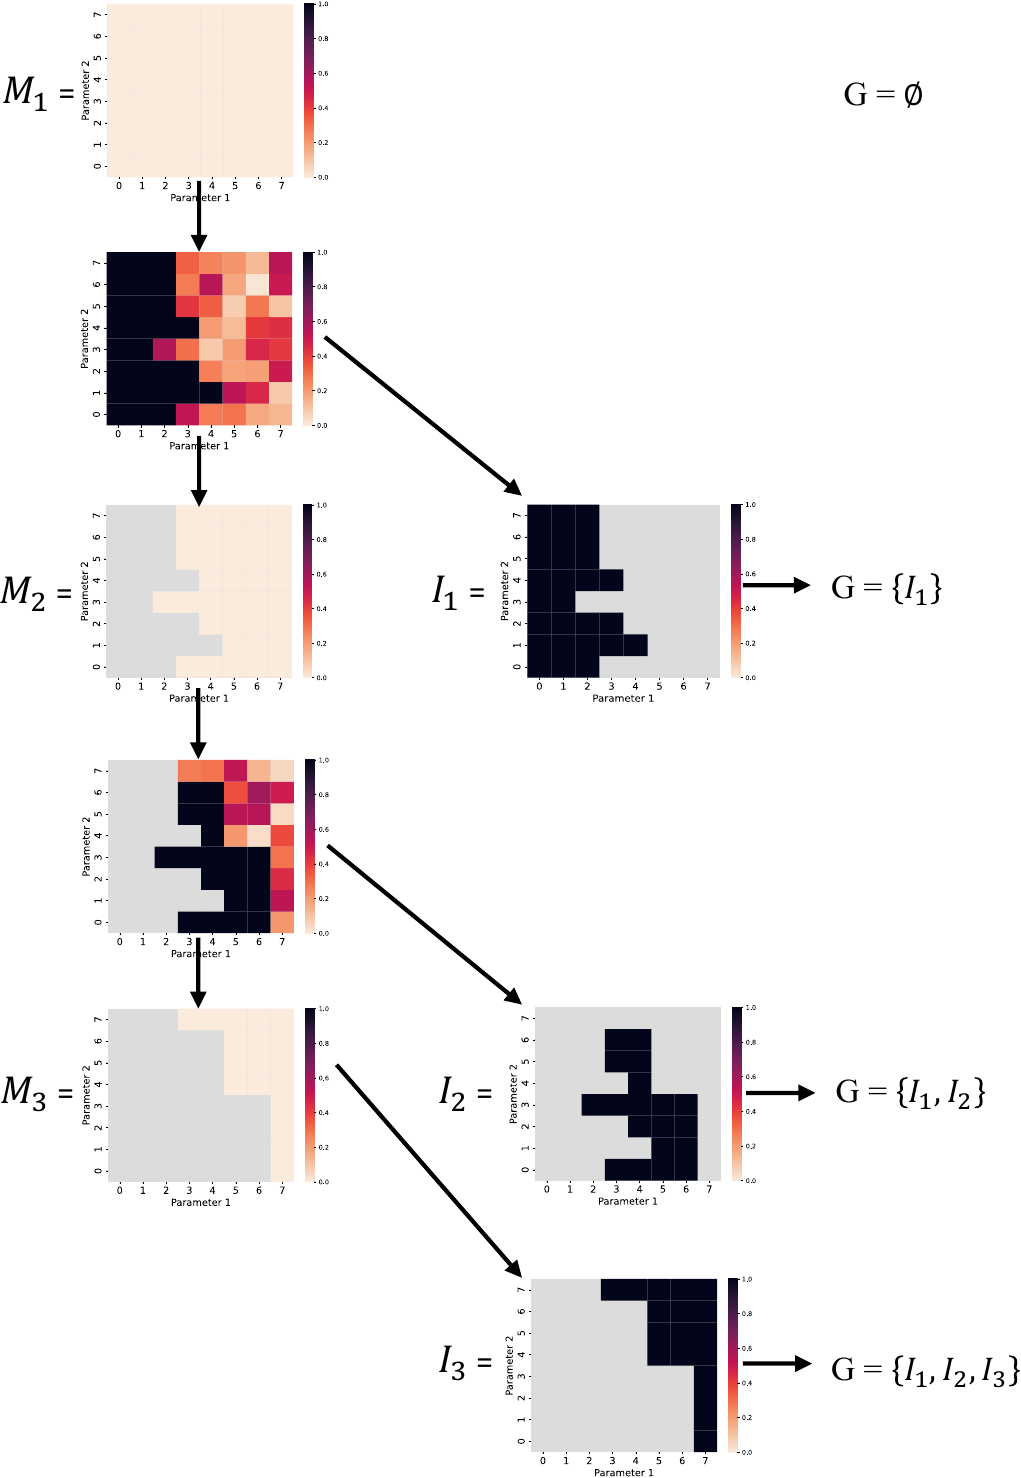}
    \caption{Visualization of an example of the evolutionary branching. The algorithm starts with an empty set $G$ and a morphology set $M_1$ which results in a controller $I_1$ and a set of left-over morphologies $M_2$. $I_1$ is added to $G$ and the evolution restarts with $M_2$. This repeats until enough  controllers $I$ have been found that together cover the morphology space and have been added to $G$. Overall, the process partitions the morphological space into clusters that can be controlled by generalist controllers as much as possible. } 
    \label{fig:visual_alg}
\end{figure*}
